# Supplementary material for: Linear Item-Item Model with Neural Knowledge for Session-based Recommendation
Source: arXiv:2504.15057 source file (2025-04-21)
Supplement: Supplementary file 1 [file sec-appendix.tex]

\newpage
\appendix\label{sec:appendix}

% \section{Limitations}\label{app:limitation}

% While the proposed method, Linear Item-Item Models with Neural Knowledge (LINK), has demonstrated notable performance, several limitations must be acknowledged. (i) Dependency on Neural Knowledge. The performance of LINK heavily relies on the quality and the relevance of the neural knowledge it incorporates. If the neural models used for extracting the regularization matrix are not well-suited or optimized, the effectiveness of LINK may be compromised. This dependence highlights the need for careful selection and tuning of neural models from which knowledge is utilized. (ii) Sensitivity to Hyperparameters. The performance of LINK is somewhat sensitive to the choice of hyperparameters, such as the regularization coefficients $\lambda$ and the temperature of neural model $\tau$. Finding the optimal set of hyperparameters can be a time-consuming process; fortunately, however, training a linear model can be done very efficiently~\cite{ChoiKLSL21SLIST, Steck19EASE} thanks to the closed-form solution. 

\section{Theoretical analysis}\label{app:Theoretical_analysis}

\subsection{Closed-form Solutions} \label{app:closed_form_solution}
We provide a detailed derivation of the closed-form solutions for
the linear knowledge-enhanced item-item similarity model (\ie, Eq.~\eqref{eq:slis_loss} and Eq.~\eqref{eq:sse_loss}) and the neural knowledge-enhanced item-item transition model (\ie, Eq.~\eqref{eq:tke_loss}).

\noindent
\subsubsection{Linear knowledge-enhanced item-item similarity model.} The objective function in Eq.~\eqref{eq:slis_loss} and Eq.~\eqref{eq:sse_loss} can be rewritten as follows.
\begin{equation}
  \label{eq:slis_loss2}
  \mathcal{L}^{\text{S}}(\mathbf{B}) = \|\mathbf{X} - \mathbf{X} \cdot \mathbf{B}\|_F^2 + \lambda \|\mathbf{B}\|_F^2 \ \text{s.t.}\ \texttt{diag}(\mathbf{B}) \le \xi
\end{equation}
\begin{equation}
  \label{eq:lis_loss2}
  \mathcal{L}^{\text{LIS}}(\mathbf{B}) = \|\mathbf{X}' - \mathbf{X}' \cdot \mathbf{B}\|_F^2 + \lambda \|\mathbf{B}\|_F^2 \ \text{s.t.}\ \texttt{diag}(\mathbf{B}) \le \xi.
\end{equation}

We derive the solution based on Eq.~\eqref{eq:slis_loss2}. Note that the same derivation process can be applied to Eq.~\eqref{eq:sse_loss} by simply replacing $\mathbf{X}$ with $\mathbf{X}'$. The final solution also only differs in using $\mathbf{X}$ versus $\mathbf{X}'$.

To solve the constrained optimization problem, we define a new objective function $\mathcal{L}^{\text{S}}(\mathbf{B}, \mathbf{\mu})$ by applying a Lagrangian multiplier and a KKT (Karush-Kuhn-Tucker) condition.
\begin{equation}
  \label{eq:slis_kkt_loss}
    \mathcal{L}^{\text{S}}(\mathbf{B}, \mu) = \| ( \mathbf{X} - \mathbf{X} \cdot \mathbf{B} )\|_F^2 + \lambda \|\mathbf{B}\|_F^2 + 2\mathbf{\mu}^{\top}\texttt{diag}(\mathbf{B} - \xi\mathbf{I}),
\end{equation}
where $\mathbf{\mu} \in \mathbb{R}^{n}$ is the KKT multiplier that satisfies $\forall \text{i}, \mathbf{\mu}_{i} \geq 0$. Then, we differentiate $\mathcal{L}^\text{S}(\mathbf{B}, \mathbf{\mu})$ with respect to $\mathbf{B}$ to minimize Eq.~\eqref{eq:slis_kkt_loss}.
\begin{align}
    \frac{1}{2}\frac{\partial \mathcal{L}^\text{S}(\mathbf{B},\mu) }{\partial \mathbf{B}}  &  \ = (-\mathbf{X}^{\top})  (\mathbf{X} - \mathbf{X} \cdot \mathbf{B}) + \lambda\mathbf{B} + \texttt{diagMat}(\mathbf{\mu}) \nonumber
  \label{eq:slis_kkt_loss_diff} \\
    & \ =    - \mathbf{X}^{\top}  \mathbf{X} + \mathbf{X}^{\top}  \mathbf{X} \cdot \mathbf{B} + \lambda\mathbf{B} + \texttt{diagMat}(\mathbf{\mu})  \nonumber \\
    & \ =   (\mathbf{X}^{\top}  \mathbf{X} + \lambda\mathbf{I})\mathbf{B} - \mathbf{X}^{\top}  \mathbf{X} +\texttt{diagMat}(\mathbf{\mu}). 
\end{align}
Therefore, we can derive $\hat{\mathbf{B}}^\text{S}$ as follows:
\begin{align}
    \hat{\mathbf{B}}^\text{S} & = (\mathbf{X}^{\top}  \mathbf{X} + \lambda\mathbf{I})^{-1} \cdot  [\mathbf{X}^{\top}  \mathbf{X}+ \lambda\mathbf{I} - \lambda\mathbf{I} -\texttt{diagMat}(\mathbf{\mu})] \nonumber\\
    & = \hat{\mathbf{P}}[\hat{\mathbf{P}}^{-1} - \lambda\mathbf{I} - \texttt{diagMat}(\mathbf{\mu}) ] \nonumber\\
    & = \mathbf{I} - \hat{\mathbf{P}}[\lambda\mathbf{I} + \texttt{diagMat}(\mathbf{\mu}) ] \nonumber \\ 
    & = \mathbf{I} - \lambda \hat{\mathbf{P}} - \hat{\mathbf{P}}\cdot \texttt{diagMat}(\mathbf{\mu}), 
    \label{eq:slis_optimal_B_derivation}
\end{align}
where $\hat{\mathbf{P}} = \left( \mathbf{X}^{\top} \mathbf{X} + \lambda\mathbf{I} \right)^{-1}$. 

A KKT multiplier $\mathbf{\mu}_{j}$ is zero only if $\mathbf{B}_{jj} \leq \xi$. Otherwise, $\mathbf{\mu}_{j}$ has a non-zero value. In this case, $\mathbf{\mu}_{i}$ regularizes the value of $\mathbf{B}_{jj}$ as $\mathbf{B}_{jj} = \xi$. For $\mathbf{B}_{jj}$, we can develop the following equation:
\begin{equation}
  \label{eq:regulate_by_mu}
  \mathbf{B}_{jj} \ = \xi = \ 1 -  \lambda P_{jj} - P_{jj}\mathbf{\mu}_{j}.
\end{equation}

Finally, $\mathbf{\mu}_{j}$ can be expressed as follows:
\begin{equation}
   \mu_{j} = \frac{(1 - \lambda P_{jj} - \xi )}{P_{jj}}
     = \frac{(1 - \xi)}{P_{jj}} - \lambda.
\end{equation}

Substituting $\mu$ in Eq.~\eqref{eq:slis_optimal_B_derivation} and enforcing non-negative elements give $\hat{\mathbf{B}}^\text{S}$:
\begin{equation}
  \label{eq:slis_solution4}
  \hat{\mathbf{B}}^\text{S} = \mathbf{I} -  \hat{\mathbf{P}} \cdot  \texttt{diagMat}(\gamma),
\end{equation}
\begin{equation}
    \label{eq:case_of_gamma_App}
    \gamma_{j} =
    \begin{cases}
        \ \ \ \lambda & \text{if} \ \ \ 1 - \lambda P_{jj} \le \xi \\
        \ \ \ \frac{1-\xi}{P_{jj}} & \text{otherwise}. 
    \end{cases}
\end{equation}

Here, $\mathbf{\gamma}$ is a vector defined by $\mathbf{\gamma} = \mathbf{\mu} + \lambda \cdot \mathbf{1}$.

\noindent
\subsubsection{Neural knowledge-enhanced item-item transition model.}
The objective function in Eq.~\eqref{eq:tke_loss} can be rewritten as follows.
\begin{equation}
  \label{eq:nit_loss4}
  \mathcal{L}^\text{NIT}(\mathbf{B}) = \|\mathbf{\Tilde{Z}} - \mathbf{\Tilde{Y}} \cdot \mathbf{B}\|_F^2 + \lambda \|\textbf{T} - \mathbf{B}\|_F^2.
\end{equation}

The first-order derivative of Eq.~\eqref{eq:nit_loss4} over $\mathbf{B}$ is as follows.
\begin{equation}
\label{eq:B_hat_of_nit}
\begin{aligned}
   \frac{1}{2} \cdot \frac{\partial \mathcal{L}^\text{NIT}}{\partial \mathbf{B}}  &  \ =  \ \ (-\mathbf{\Tilde{Y}}^{\top}){(\mathbf{\Tilde{Z}} - \mathbf{\Tilde{Y}} \cdot \mathbf{B})} + \lambda (\mathbf{B} - \textbf{T}), \\
    & \ =  \ \  (\mathbf{\Tilde{Y}}^{\top} \mathbf{\Tilde{Y}} + \lambda\mathbf{I})\cdot\mathbf{B} - \mathbf{\Tilde{Y}}^{\top} \mathbf{\Tilde{Z}} - \lambda\textbf{T}.
\end{aligned}
\end{equation}

So, the closed-form solution of Eq.~\eqref{eq:nit_loss4} is as follows.
\begin{equation}
  \label{eq:slit_solution4}
  \hat{\mathbf{B}}^\text{NIT} \ = (\mathbf{\Tilde{Y}}^{\top} \mathbf{\Tilde{Y}} + \lambda \mathbf{I})^{-1} \cdot (\mathbf{\Tilde{Y}}^{\top} \mathbf{\Tilde{Z}} + \lambda \textbf{T} ).
\end{equation}

\section{Additional Experimental Setup}

\begin{table}[]
\centering
\caption{Optimal hyperparameters of LINK for each dataset.}\label{tab:optimal_hyper}
\begin{tabular}{c|cccccc}
\toprule
Dataset & $\alpha$ & $\beta$ & $\lambda$ & $\tau$ & $\delta_{\text{pos}}$ & $\delta_{\text{inf}}$ \\
\midrule
Diginetica & 0.9 & 1.0 & 10$^2$ & 0.1 & 1.0 & 4.0 \\
Retailrocket & 0.9 & 0.9 & 10$^2$ & 0.1 & 1.0 & 4.0 \\
Yoochoose & 0.5 & 1.0 & 10$^3$ & 0.1 & 1.0 & 1.0 \\
Tmall & 0.9 & 1.0 & 10$^3$ & 0.05 & 1.0 & 4.0 \\
Dressipi & 0.9 & 0.5 & 10$^2$ & 0.1 & 1.0 & 4.0 \\
LastFM & 0.9 & 1.0 & 10$^2$ & 0.1 & 1.0 & 8.0 \\
% \midrule
% Beauty & 0 & 100 & - & 1.0 & 1.0 \\
% Toys & 0 & 200 & - & 1.0 & 1.0 \\
% Sports & 0 & 1000 & - & 1.0 & 1.0 \\
% Yelp & 0.7 & 200 & 1 & 2.0 & 2.0 \\
\bottomrule
\end{tabular}
\end{table}

\subsection{Optimal Hyperparameters}\label{app:optimal_hyper}
Table~\ref{tab:optimal_hyper} shows the tuned hyperparameters of LINK for the following datasets: Diginetica, Retailrocket, Yoochoose, Tmall, Dressipi, and LastFM.

\section{Additional Experimental Results}\label{app:results}

\subsection{Hyperparameter Study}\label{app:hyperparameter_study}
\begin{figure*}[t]\small
\centering
\includegraphics[width=1.0\linewidth]{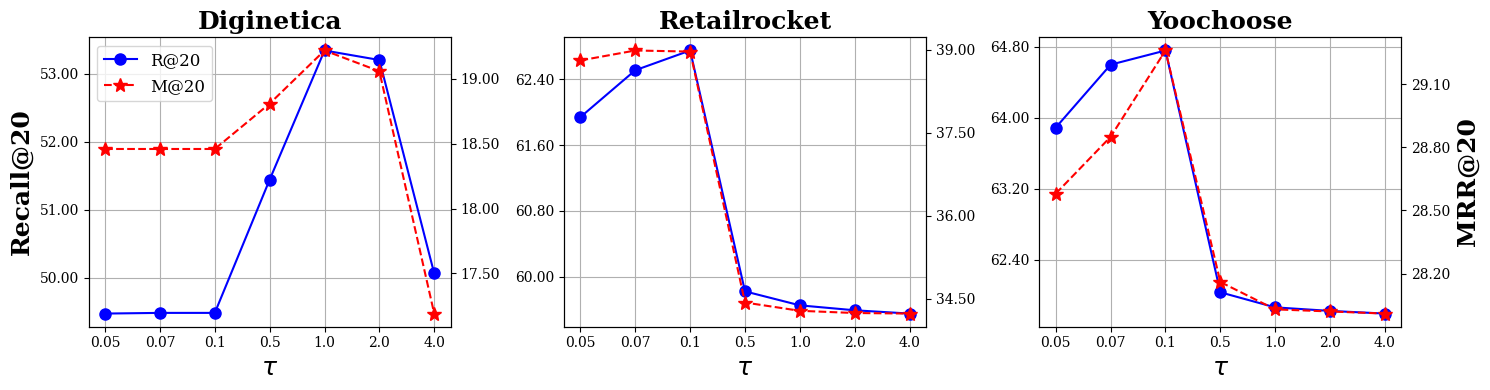}
\caption{Performance of LINK over varying temperature $\tau$.}\label{fig:exp_teacher_tau}
\vspace{-3mm}
\end{figure*}

\iffalse

\begin{figure}[t]
\centering
\begin{tabular}{ccc}
\includegraphics[width=0.3\textwidth]{Figures/fig_length_diginetica.png}  &
\includegraphics[width=0.3\textwidth]{Figures/fig_length_diginetica.png}  & 
\includegraphics[width=0.3\textwidth]{Figures/fig_length_diginetica.png}  
\\
(a) Diginetica & (b) Retailrocket & (c) Yoochoose \\
\end{tabular}
\caption{Performance of LINK over varied temperature $\tau$.}\label{fig:exp_teacher_tau}
\vspace{-3mm}
\end{figure}

\fi
\begin{figure*}[t]\small
\centering
\includegraphics[width=1.0\linewidth]{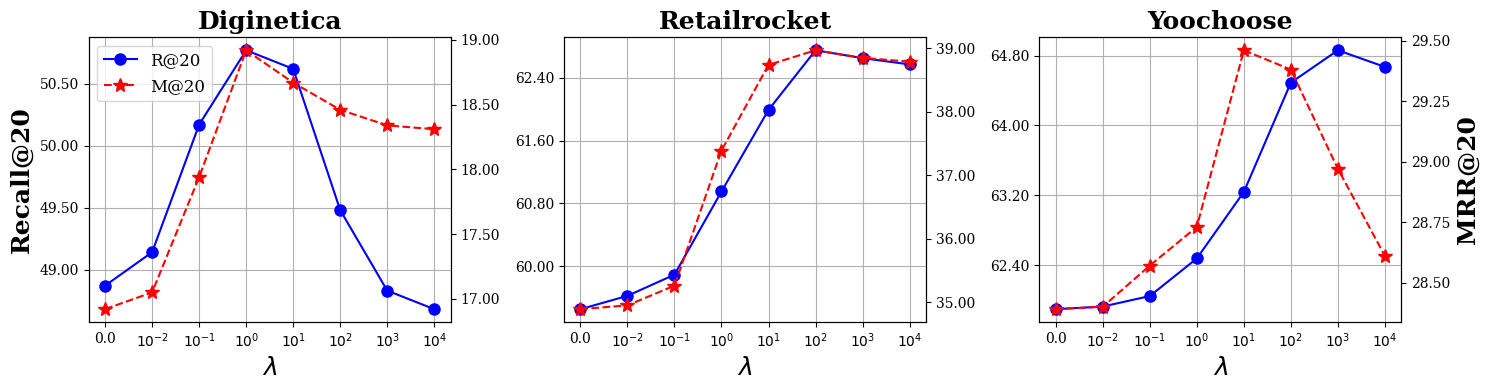}
\caption{Performance of LINK over varying regularization coefficient $\lambda$.}\label{fig:exp_teacher_beta}
\vspace{-3mm}
\end{figure*}

Figure~\ref{fig:exp_teacher_tau} and \ref{fig:exp_teacher_beta} show the performance of LINK depending on the temperature $\tau$ in Eq.~\eqref{eq:teacher_single_item} and the regularization hyperparameter $\lambda$ in Eq.~\eqref{eq:tke_loss} on Diginetica, Retailrocket and Yoochoose datasets. For Retailrocket and Yoochoose datasets, LINK achieves optimal performance with temperature $\tau$ values of 0.07 or 0.1. On the other hand, LINK performs best with a $\tau$ value of 1 for Diginetica dataset, highlighting that optimal hyperparameters can vary significantly across datasets.

For the regularization hyperparameter $\lambda$, the optimal values based on MRR@20 are 1, $10^2$, and 10 for Diginetica, Retailrocket, and Yoochoose, respectively. For Retailrocket and Yoochoose, the use of relatively larger $\lambda$ values for regularizing the neural teacher matrix proves to be particularly effective.
