# Supplementary material for: Linear Item-Item Model with Neural Knowledge for Session-based Recommendation
Source: arXiv:2504.15057 source file (2025-04-21)
Supplement: Supplementary file 2 [file Fig_flops_appendix.tex]

\begin{figure*}
\begin{tabular}{cc}
\includegraphics[width=0.48\linewidth]{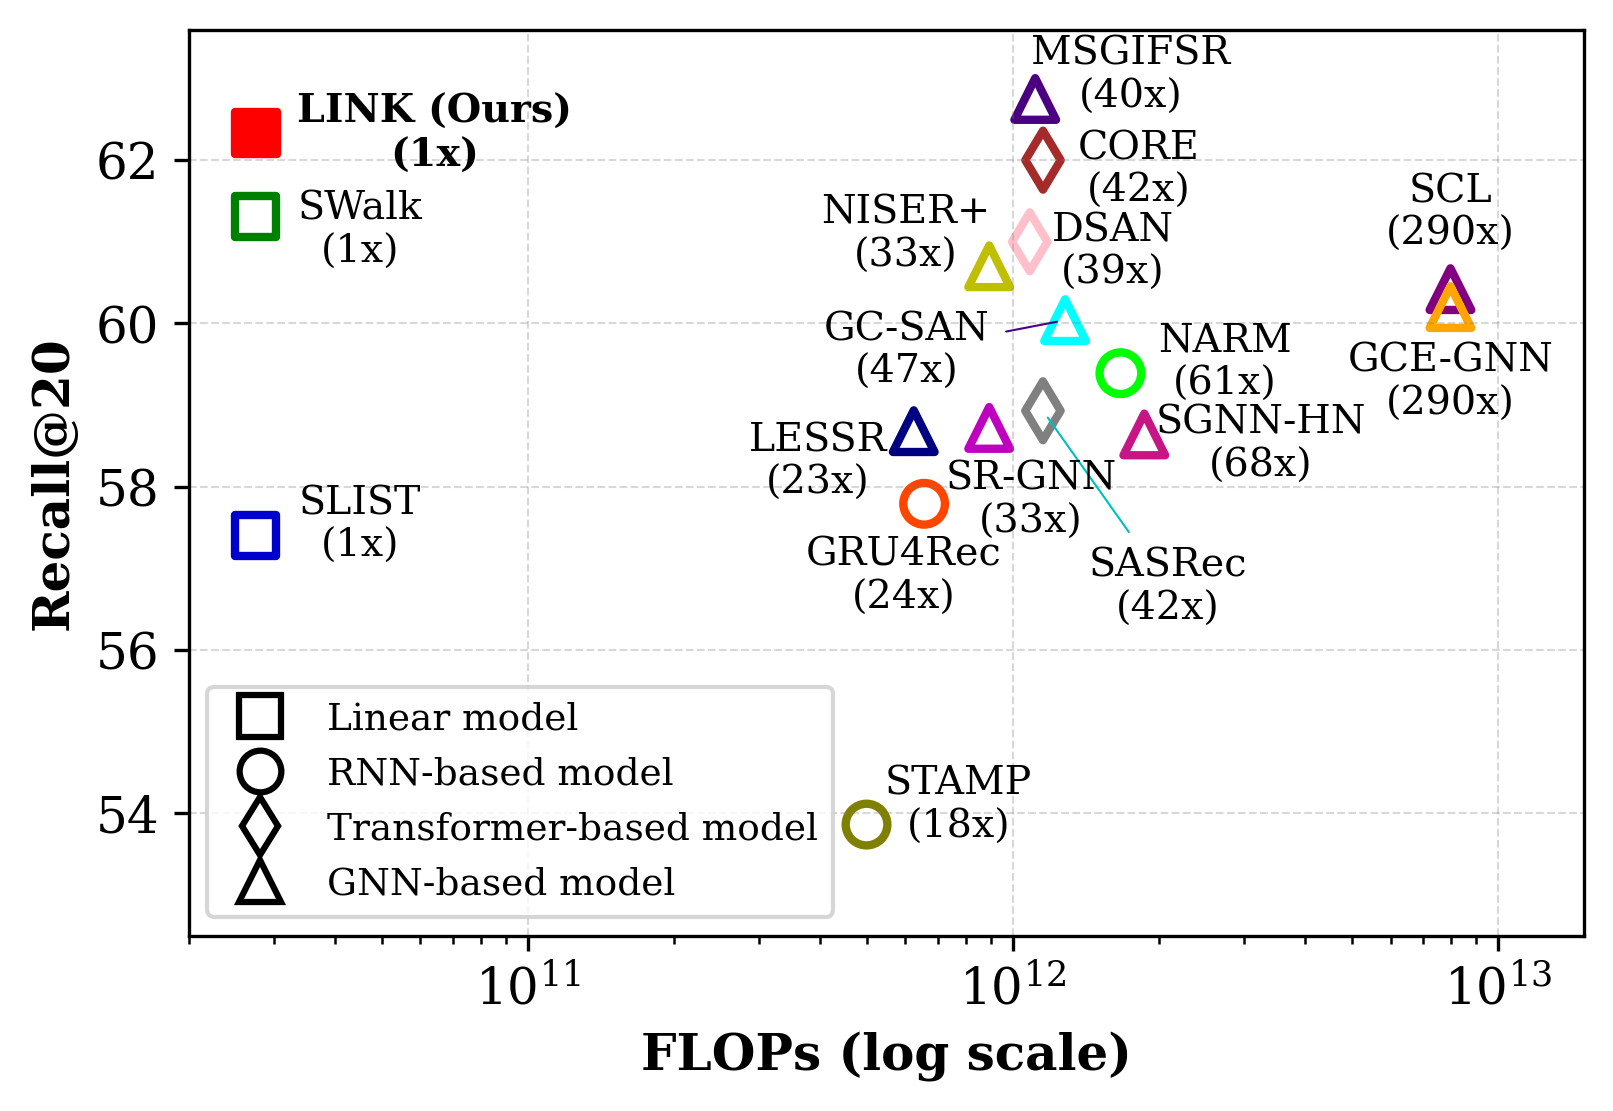} 
& \includegraphics[width=0.48\linewidth]{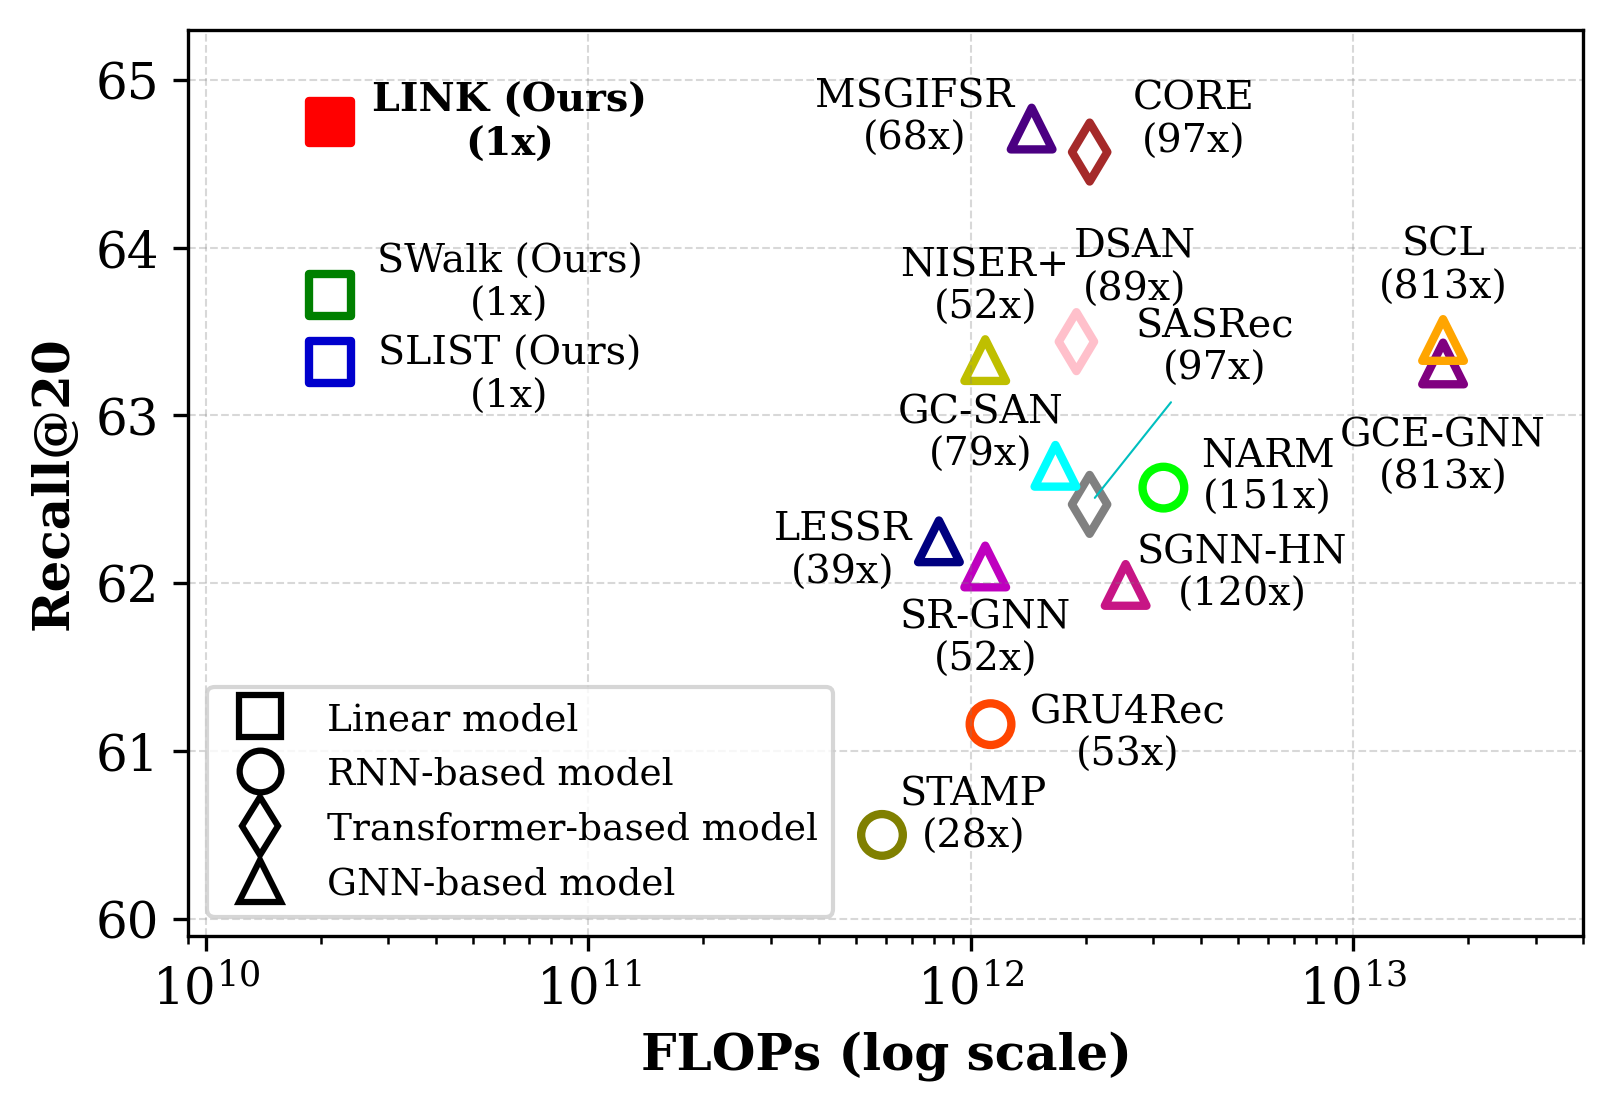}  \\
(a) Retailrocket & (b) Yoochoose
\end{tabular}
\caption{Performance comparison over the Recall@20 and the log-scaled number of floating point operations (FLOPs) for inference on Retailrocket and Yoochoose datasets. The numbers in parentheses indicate the relative FLOPs compared to LINK.}\label{fig:exp_flops_appendix}
\Description{}{}
\end{figure*}

\iffalse
% -- Two columns figure --

\begin{figure*}
\begin{tabular}{cc}
\includegraphics[width=0.4\linewidth]{Figures/digi_flops_recall.png} 
& \includegraphics[width=0.4\linewidth]{Figures/yc_flops_recall.png}  \\
(a) Diginetica & (b) Yoochoose
\end{tabular}
\caption{Performance comparison over the Recall@20 and the number of floating point operations for inference. The numbers in parentheses indicate the multiple of FLOPs compared to LINK.}\label{fig:exp_flops}
\Description{}{}
\end{figure*}
% The square marker indicates a linear model. The circle, triangle, and diamond markers indicate RNN-, GNN-, and transformer-based neural models, respectively.

\fi
